# Supplementary material for: Two-Stage Random Alternation Framework for One-Shot Pansharpening
Source: arXiv:2505.06576 source file (2025-05-16)
Supplement: Supplementary file 1 [file 12_appendix.tex]

\section{Complexity Analysis of MLP Architecture}
\label{sec:appendix_section}
Our MLP design consists of 3 layers, with a hidden layer size of 32 and the Sigmoid activation function. This simple architecture is intentionally chosen to prevent overfitting, especially in data-scarce zero-shot scenarios. Despite its simplicity, the MLP effectively captures the required degradation relationships, and the experimental results demonstrate its excellent performance.
\begin{figure}[htp]
    \centering
    \includegraphics[width=1.0\linewidth]{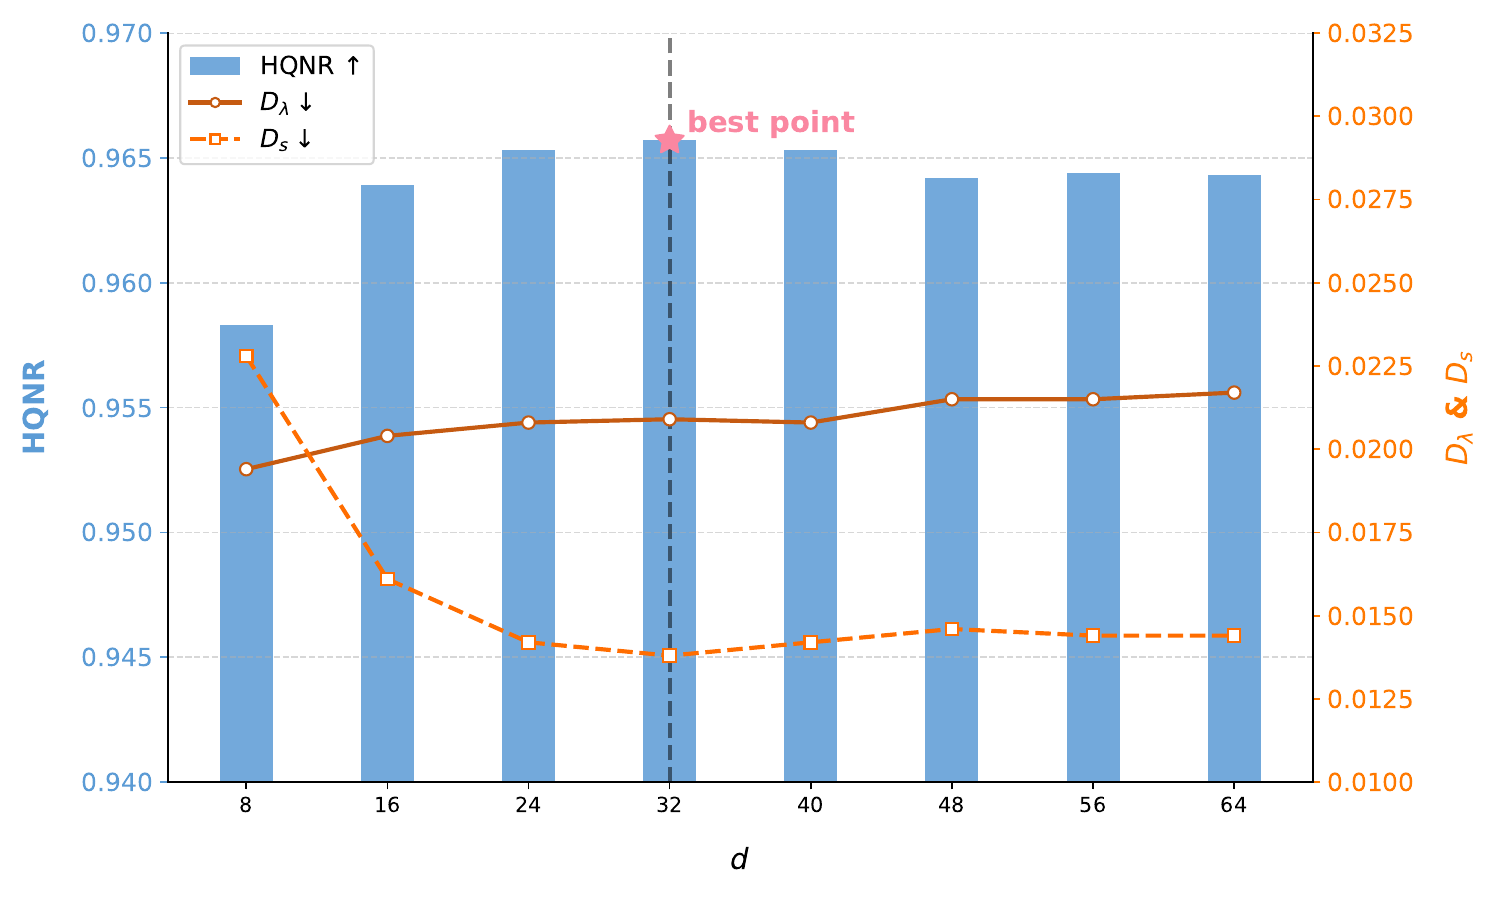}
    \vspace{-20pt}
    \caption{
  Effect of hidden layer size \(d\) on HQNR during training.
    }
\end{figure}

In this study, we conducted a systematic experiment on the architectural selection of Multilayer Perceptron (MLP) networks, providing quantitative support for the rational design of MLP structures. We focused on investigating the impact of hidden layer size \(d\) on model complexity and performance. The experiments were conducted on the WV3 dataset, ensuring strict control of variables by keeping other hyperparameters constant. A line plot illustrates the training performance trends across different representative values of \(d\) as a function of training epochs. The results indicate that when the hidden layer size is small, the network's expressiveness is limited, leading to insufficient modeling capability of the DAM degradation process and ultimately poor performance. As dd increases to the optimal value of 32, the network achieves a balance between fitting capacity and generalization ability, significantly enhancing the simulation performance. However, beyond this optimal scale, further increases in model complexity lead to overfitting, degrading generalization ability and ultimately deteriorating training performance.

\section{Explanation of MTF-matched filters}
\label{sec:MTF}
The MTF \cite{aiazzi2006mtf,vivoneContrastErrorBasedFusion2014} matching filter is used to downsample PAN, MS, and HRMS images. The MTF is primarily employed to design a low-pass filter that matches the actual response of the MS sensor, thereby more realistically simulating the low-frequency information captured by the sensor during the downsampling process. The image degradation process can be expressed as follows:
\begin{equation}
Y = (X \otimes K)\downarrow_r + n_1
\end{equation}
In this equation, the symbol \(\otimes\) denotes the convolution operation, which is used to apply the blur kernel \(K\). The blur kernel \(K \in \mathbb{R}^{k \times k}\) is a preset filter whose parameters, such as the standard deviation \(\sigma\), are determined based on the sensor's gain at the Nyquist frequency to match the actual MTF of the sensor. The operator \(\downarrow_r\) indicates down-sampling by a factor of \(r\). Additionally, \(n_1\) represents a small residual value, typically modeled by a zero-mean Gaussian distribution, which accounts for noise during the degradation process.
This filter typically has a Gaussian-like shape, and its sole free parameter, the standard deviation, is set according to the sensor's gain at the Nyquist frequency, allowing it to closely match the MS sensor’s MTF. By employing this filter in our network, we are able to more accurately simulate the sensor characteristics associated with resolution degradation when changing data scales.

\section{Details of Data Augmentation}
\label{sec:DA}
During the DAM and RAO stages of the reduced-resolution training, we applied data augmentation techniques. Specifically, we employed the Tencrop method, which extracts five fixed-position crops from the image. These five crops correspond to the top-left corner, top-right corner, bottom-left corner, bottom-right corner, and the center region of the image. Then, each of these five cropped regions is subjected to horizontal flipping, resulting in a dataset composed of 10 cropped images. In the zero-shot scenario, data augmentation further helps prevent the potential overfitting of the model.

\section{Analysis of Sampling Ratio}

\begin{figure}[htp]
    \centering
    \includegraphics[width=1.0\linewidth]{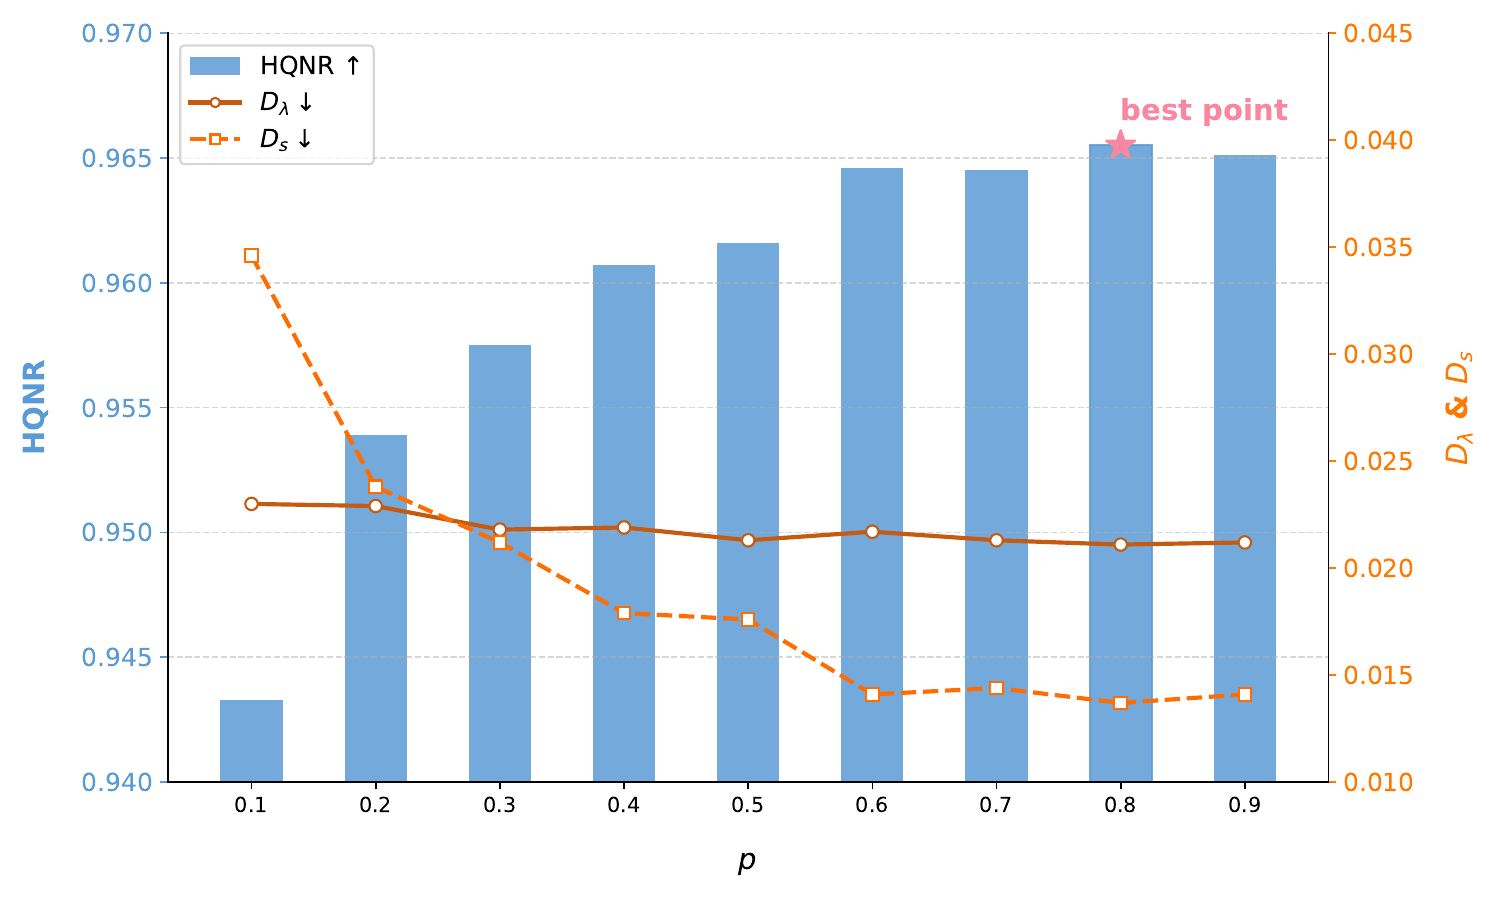}
    \vspace{-20pt}
    \caption{
  Effect of random sampling ratio \(p\) on HQNR during training.
    }
    \label{fig:ratio_sampling}
\end{figure}
Similar to the warmup epoch number \(m\), the random sampling ratio \(p\) is another critical variable in our approach, indicating the probability of inserting full-resolution training in each epoch. Likewise, we performed experiments on the WV3 dataset, maintaining all other hyperparameters constant. As illustrated in \cref{fig:ratio_sampling}, as the ratio \(p\) increases from 0.1 to 0.8, the model becomes more effective in combining the strengths of both full-resolution and reduced-resolution training. When \(p\) reaches 0.8, the best balance is achieved, resulting in optimal performance. However, as \(p\) increases further, the model is subjected to insufficient pixel-level supervision, which affects its ability to preserve spatial information, resulting in a slow decline in HQNR.

\begin{figure}[htp]
    \centering
    \includegraphics[width=1.0\linewidth]{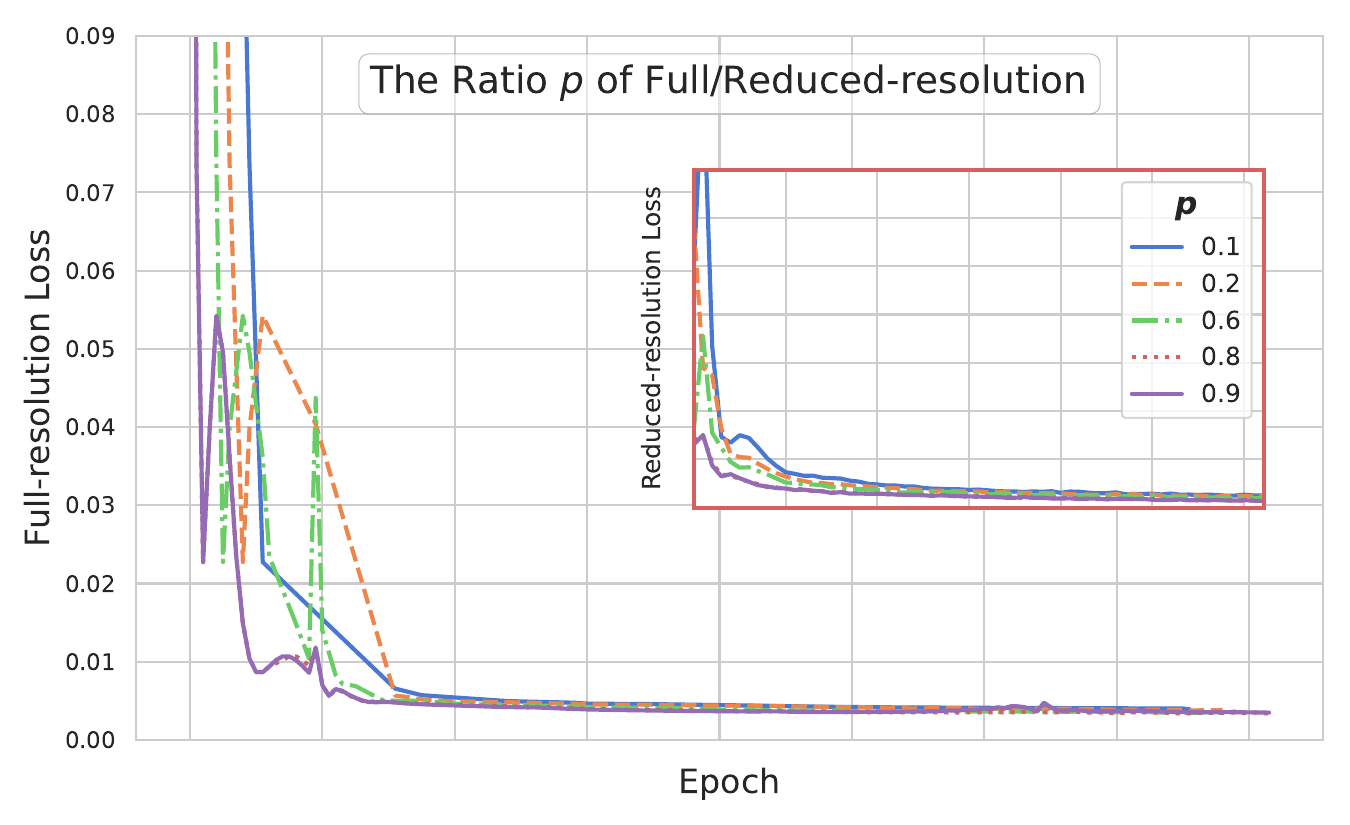}
    \vspace{-20pt}
    \caption{
Effect of the ratio \( p \) on the loss of the fusion network during Full/Reduced-resolution training.
    }
    \label{fig:ratio_loss}

\end{figure}
This study further explores the role of the random sampling ratio \( p \) in both full-resolution and downsampled-resolution training, analyzing its impact on the model optimization process through loss curve evaluations. Experimental results indicate that when training with full resolution, an excessively small \( p= 0.1 \) prevents the model from fully leveraging high-resolution information, leading to an over-reliance on downsampled features. Consequently, the training process is prone to local optima, resulting in a slow decline in loss. Even a slight increase in \( p = 0.2 \)  fails to effectively mitigate this issue and instead introduces instability in loss reduction.  d
When \( p \) is increased to 0.8, the dominant role of full-resolution features is effectively balanced with the auxiliary benefits of downsampled information, leading to a more efficient and stable training process that achieves optimal performance. Furthermore, a comparison with \( p = 0.6 \) reveals that at \( p = 0.8 \), the model exhibits greater robustness to the introduction of downsampled features after the warmup phase, further optimizing the convergence trajectory. However, when \( p \) is further increased to 0.9, the supplementary benefits of downsampled information diminish, leading to increased fluctuations in the later stages of training, ultimately compromising the convergence quality.

\section{Details on Experiments and Discussion}

\subsection{Datasets}
We conducted experiments on data collected from the WorldView-3 (WV3), QuickBird (QB), and GaoFen-2 (GF2) satellites. The datasets consist of images cropped from entire remote sensing images, divided into training and testing sets. The training set comprises PAN/MS/GT image pairs obtained by downsampling simulation, with dimensions of $64\times64$, $16\times16\times C$ and $64\times64\times C$, respectively.
The WV3 training set contains approximately 10,000 pairs of eight-channel images ($C = 8$), while the QB training set contains around 17,000 pairs of four-channel images ($C = 4$). GF2 training set has about 20,000 pairs of four-channel images ($C = 4$). The reduced-resolution testing set for each satellite consists of 20 downsampling simulated PAN/MS/GT image pairs with various representative land covers, with dimensions of $256\times256$, $64\times64\times C$, and $256\times256\times C$, respectively.
The full-resolution test set includes 20 pairs of original PAN/MS images with dimensions of $512 \times 512$ and $128 \times 128$. Our datasets and data processing methods are downloaded from the PanCollection repository \cite{dengMachineLearningPansharpening2022}.

\subsection{Training Details}
For training TRA-PAN on the WV3 dataset, we employed the $\ell_2$ loss function and the Adam optimizer \cite{Adam} during training. We chose a ratio of 0.8 for the RAO phase of training. In full-resolution training, the initial learning rate was set to 0.0005 and was reduced to the order of $10^{-3}$ after 250 epochs. For downsampled training, the initial learning rate remained at 0.0005 but was decreased to the order of $10^{-4}$ after 400 epochs. The total training duration for both settings was 250 epochs.
During the DAM stage, the learning rate was set to 0.0005. Regarding the network architecture, the number of channels in the hidden layers was configured to 32.
For the QB dataset, we adjusted the warm-up period to five iterations and modified the ratio to 0.7, while keeping all other parameters identical to those used for the WV3 dataset.
For the GF2 dataset, the warm-up period was extended to 80 iterations, with all other parameters remaining consistent with those used for the WV3 dataset.

% When training TRA-Net on the WV3 dataset,During the RAO stage, we utilized the $\ell_2$ loss function and Adam optimizer \todo{cite}\cite{Adam} with a batch size of 250. The initial learning rate was set at $10^{-3}$, which was reduced to $10^{-4}$ after 250 epochs. The total duration of the training was 500 epochs. Regarding the network architecture, we set the number of channels in the hidden layers to 32, the number of clusters $K$ during training was set to 32 and the threshold $\eta$ was 0.005. To encourage stable clustering learning, we recalculated and updated the cluster indices every 10 epochs during training. 

% For the QB dataset, we maintained a constant learning rate of $5 \times 10^{-4}$ and only trained for 200 epochs, while all other parameters were kept the same as in the WV3 dataset.

% \input{tables/suppl_method}

\subsection{Replacing Fusion Network Backbone}
In this section, we replaced the fusion network used in the RAO stage with LAGNet, LGPNet, and FusionNet as the backbone of our network. From \cref{table:Backbone}, we found that using LAGNet and LGPNet significantly degraded the fusion results. This is because in a zero-shot scenario, complex networks are more prone to overfitting.
\begin{table}[t]
\centering
\caption{Experiment of different backbones in WV3 dataset.}
\setlength{\tabcolsep}{4pt} % 默认值为6pt，调整为4pt以缩短列间距
\centering
\begin{tabular}{cccc}
\hline
\multirow{2}{*}{\textbf{Backbone}} & \multicolumn{3}{c}{\textbf{WV3}} \\
\cmidrule(lr){2-4}
& \textbf{D$_\lambda \downarrow$} & \textbf{D$s$$\downarrow$} & \textbf{HQNR$\uparrow$} \\
\hline
TRA-PAN  & 0.0193  & 0.0154 & 0.9657 \\
LAG  & 0.0939  &  0.1065 &  0.8103  \\
LGP & 0.0710 & 0.1408  & 0.7988  \\
\hline
\end{tabular}
\label{table:Backbone}
\end{table}

\subsection{Additional Results}
 In the following figures, we present a comparison of the visualisation outputs of the various methods on sample images from the WV3, QB, and GF2 datasets, including the residuals between the outputs at full resolution versus the HQNR images, the outputs of the reduced resolution samples and the ground truth.

\begin{figure*}[b]
   \centering
   \includegraphics[width=1.0\linewidth]{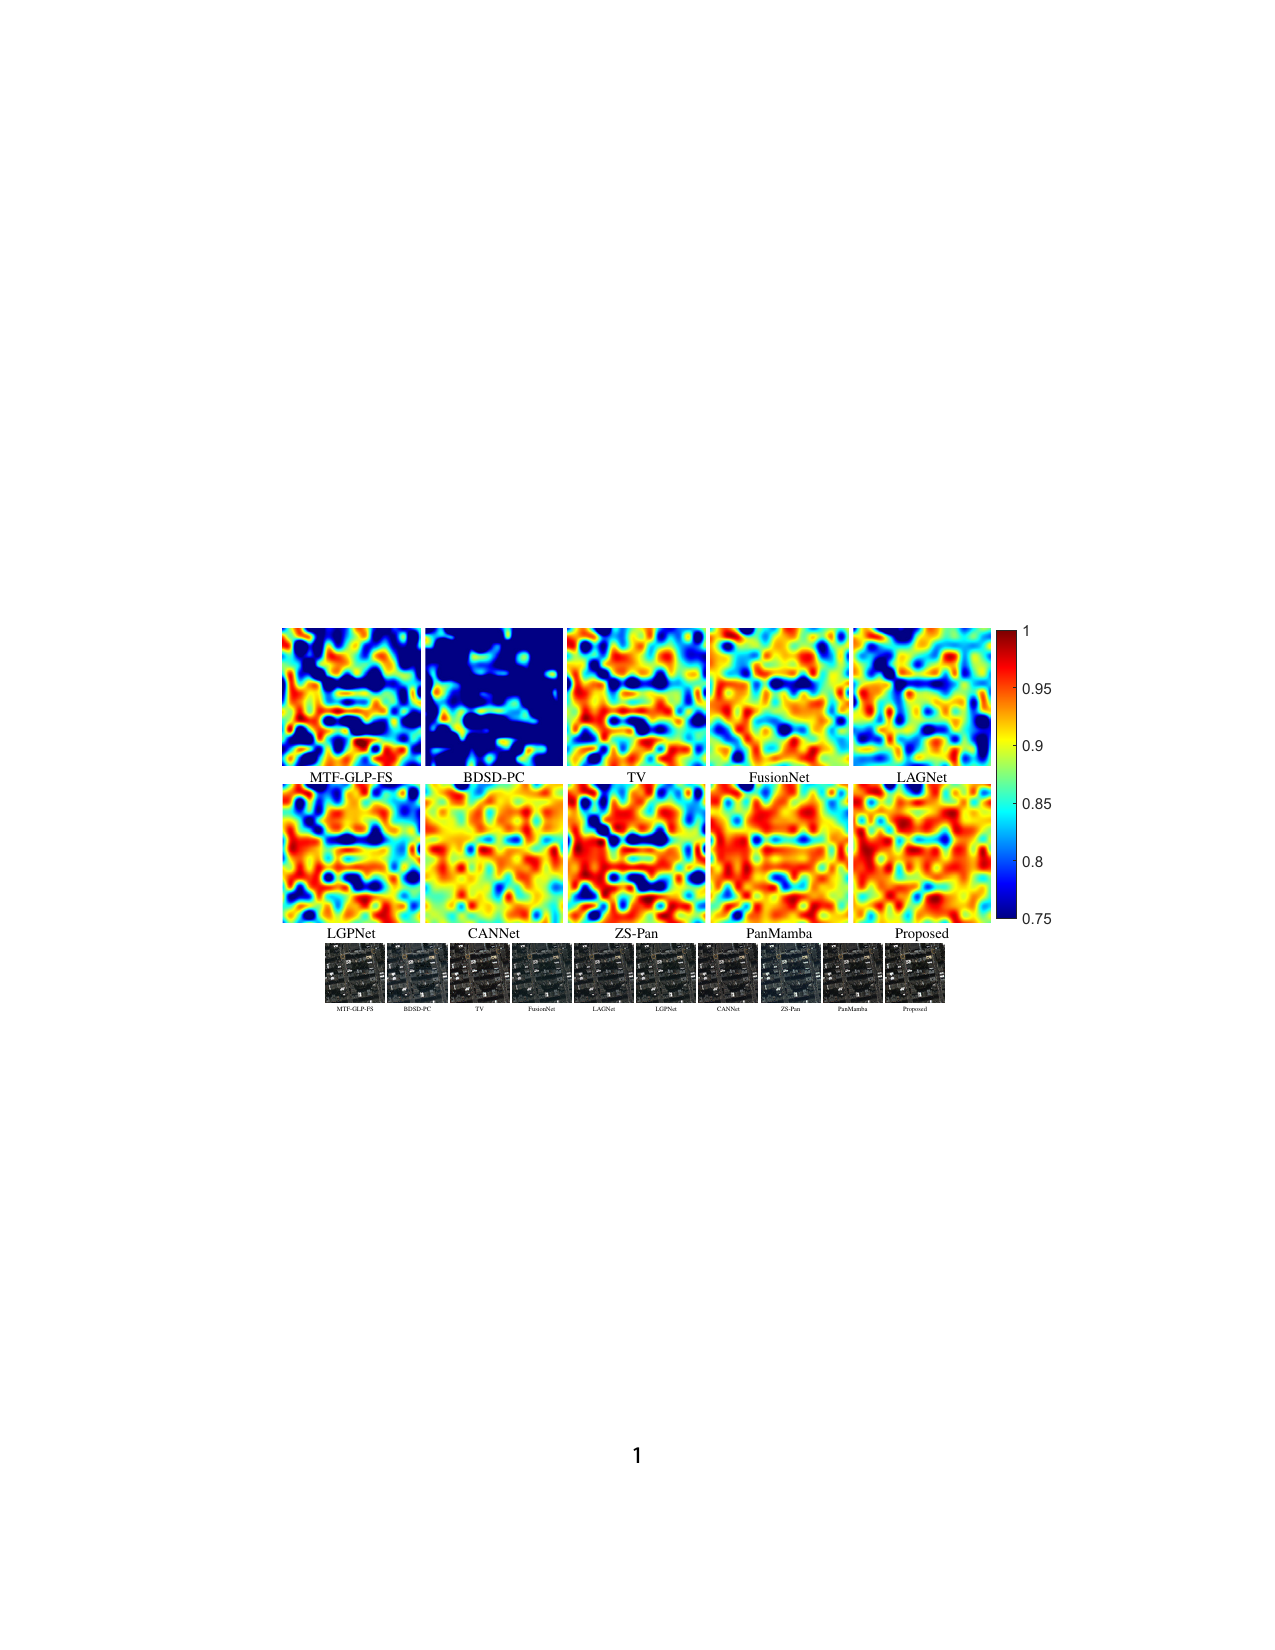}
   \vspace{-20pt}
   \caption{
 The HQNR maps (Top) and visual results (bottom) of all compared approaches on the QB full-resolution dataset.
   }
\vspace{-10pt}
\end{figure*}

\begin{figure*}[t]
   \centering
   \includegraphics[width=1.0\linewidth]{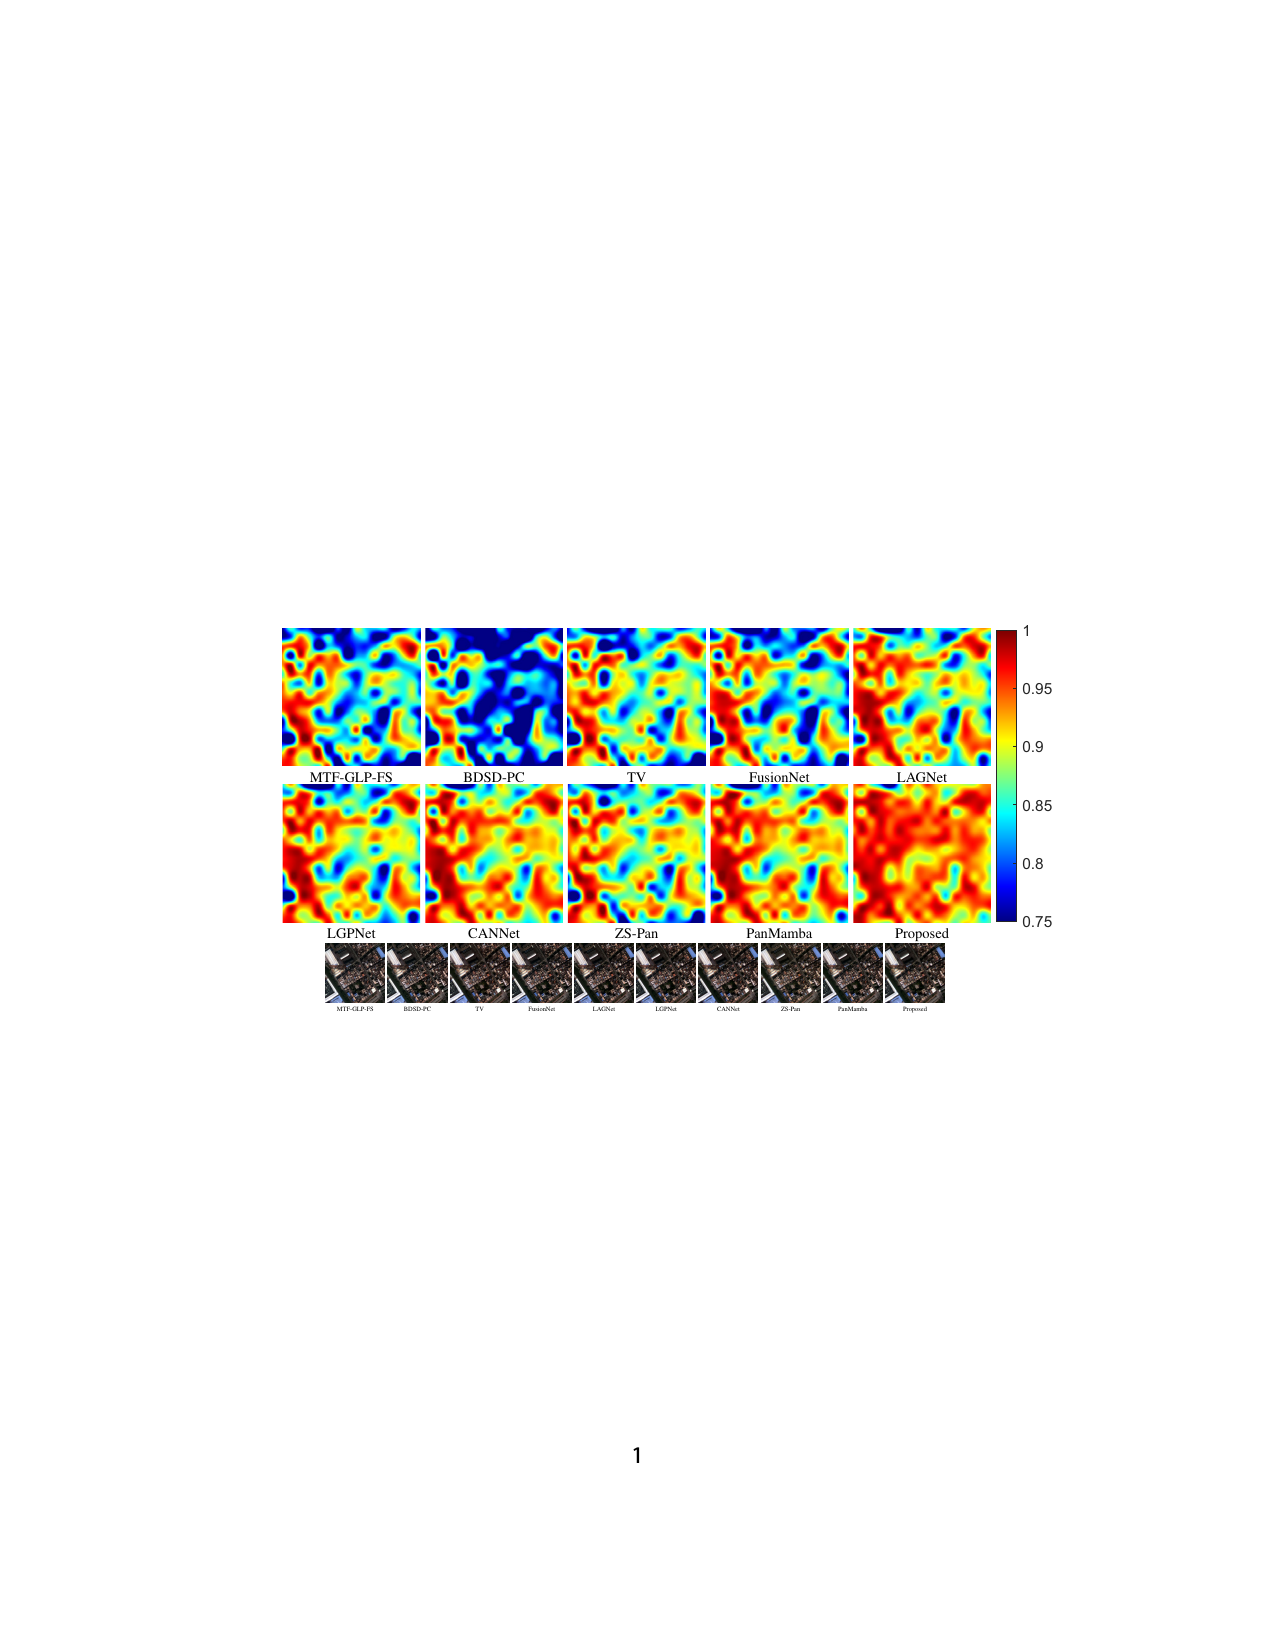}
   \vspace{-20pt}
   \caption{
  The HQNR maps (Top) and visual results (bottom) of all compared approaches on the GF2 full-resolution dataset.
   }
   \vspace{-18pt}
\end{figure*}

\begin{figure*}[t]
   \centering
   \includegraphics[width=1.0\linewidth]{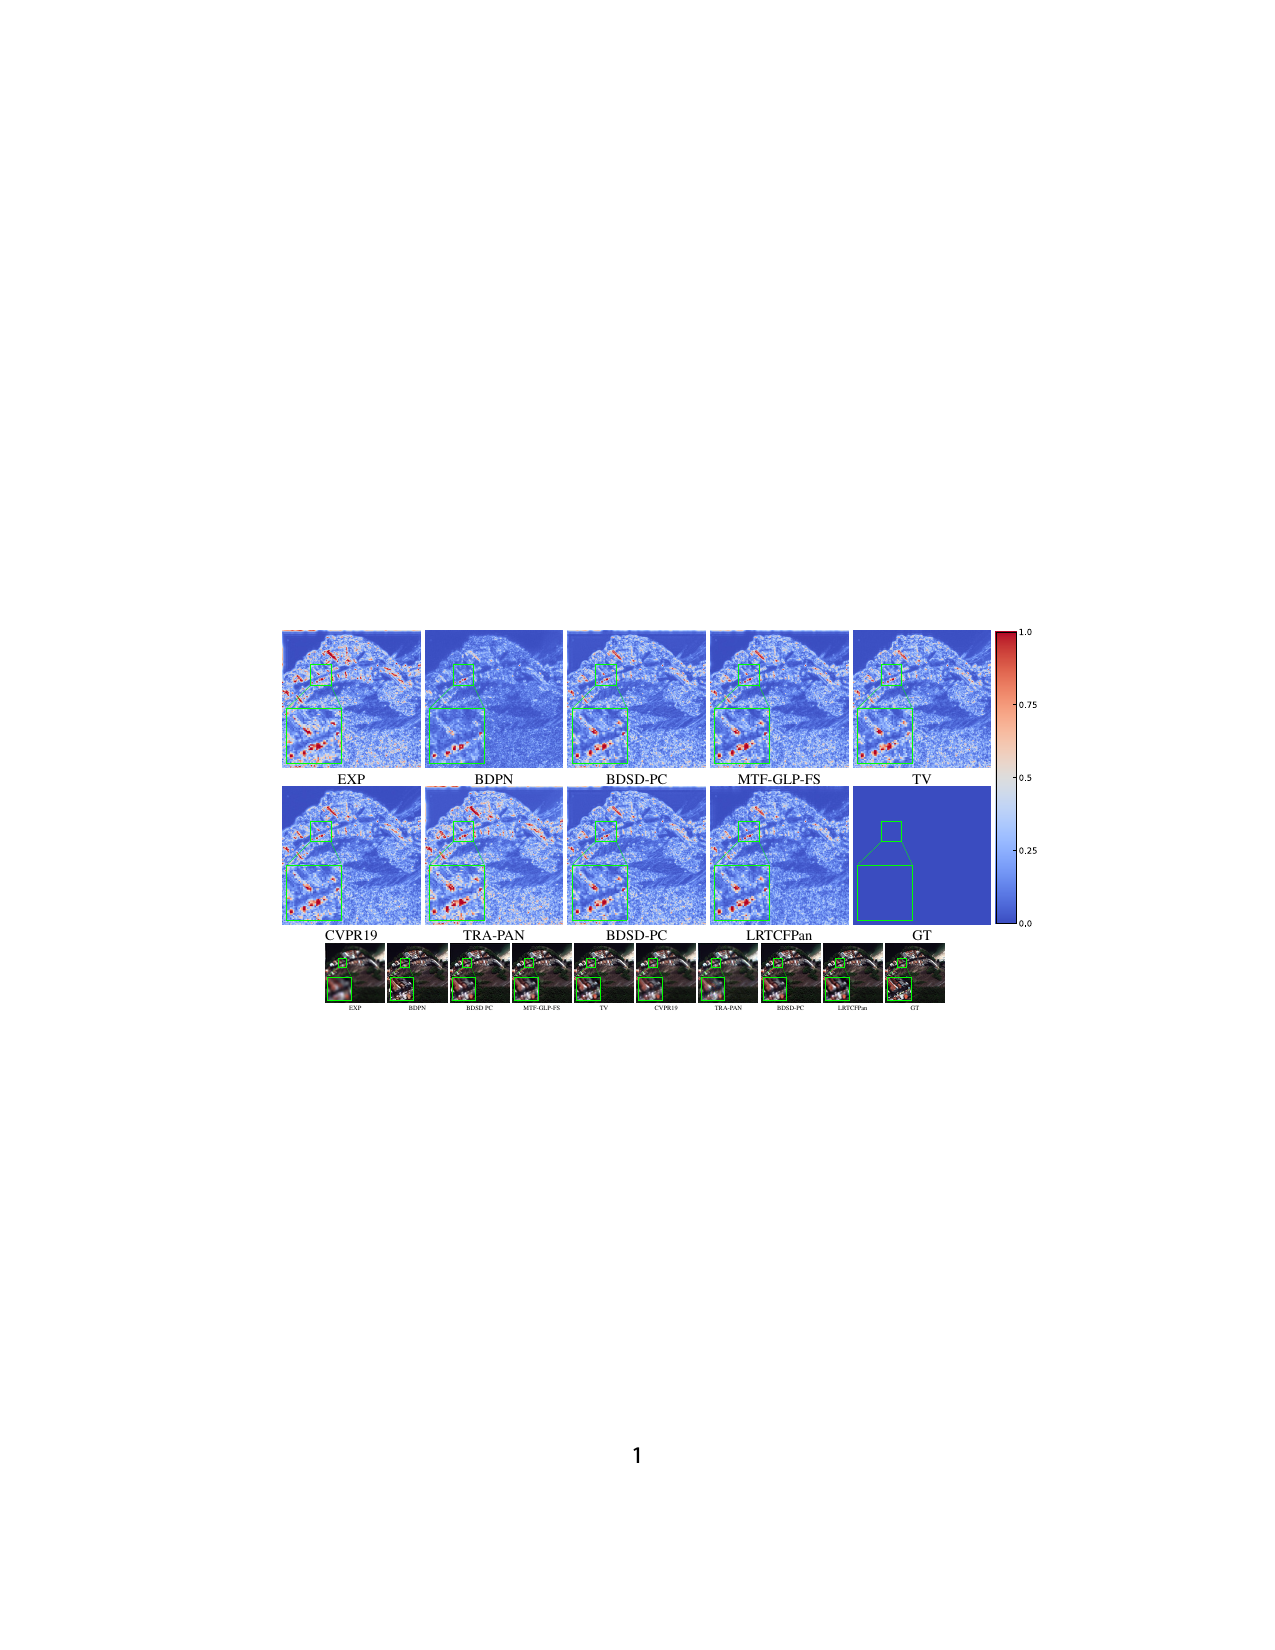}
   \vspace{-20pt}
   \caption{
  Qualitative result comparison between benchmarked methods on the sample image from WV3 reduced-resolution dataset. The
 first row presents the residual compared to the ground truth, while the second row shows  RGB outputs.
   }
   \vspace{-18pt}
\end{figure*}

\begin{figure*}[t]
   \centering
   \includegraphics[width=1.0\linewidth]{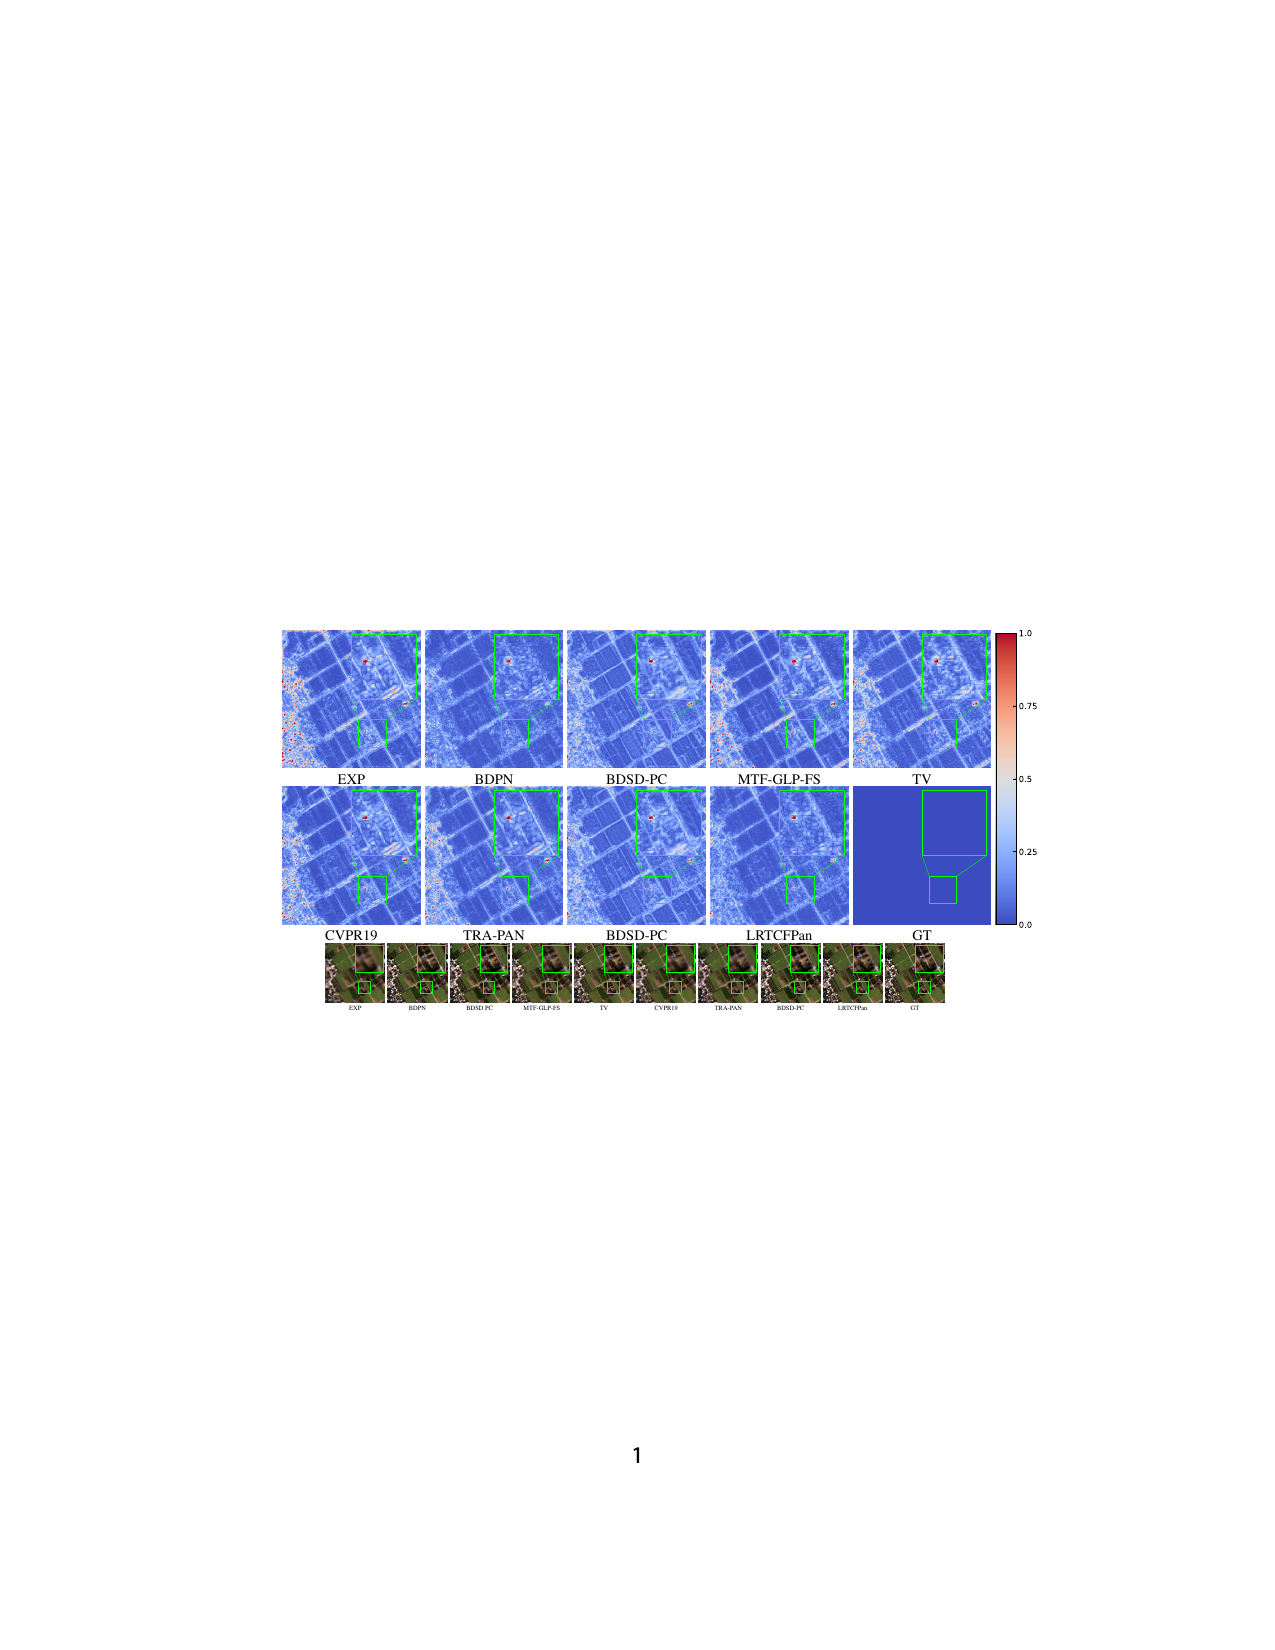}
   \vspace{-20pt}
   \caption{
 Qualitative result comparison between benchmarked methods on the sample image from GF2 reduced-resolution dataset. The
 first row presents the residual compared to the ground truth, while the second row shows  RGB outputs.
   }
   \vspace{-18pt}
\end{figure*}

\begin{figure*}[t]
   \centering
   \includegraphics[width=1.0\linewidth]{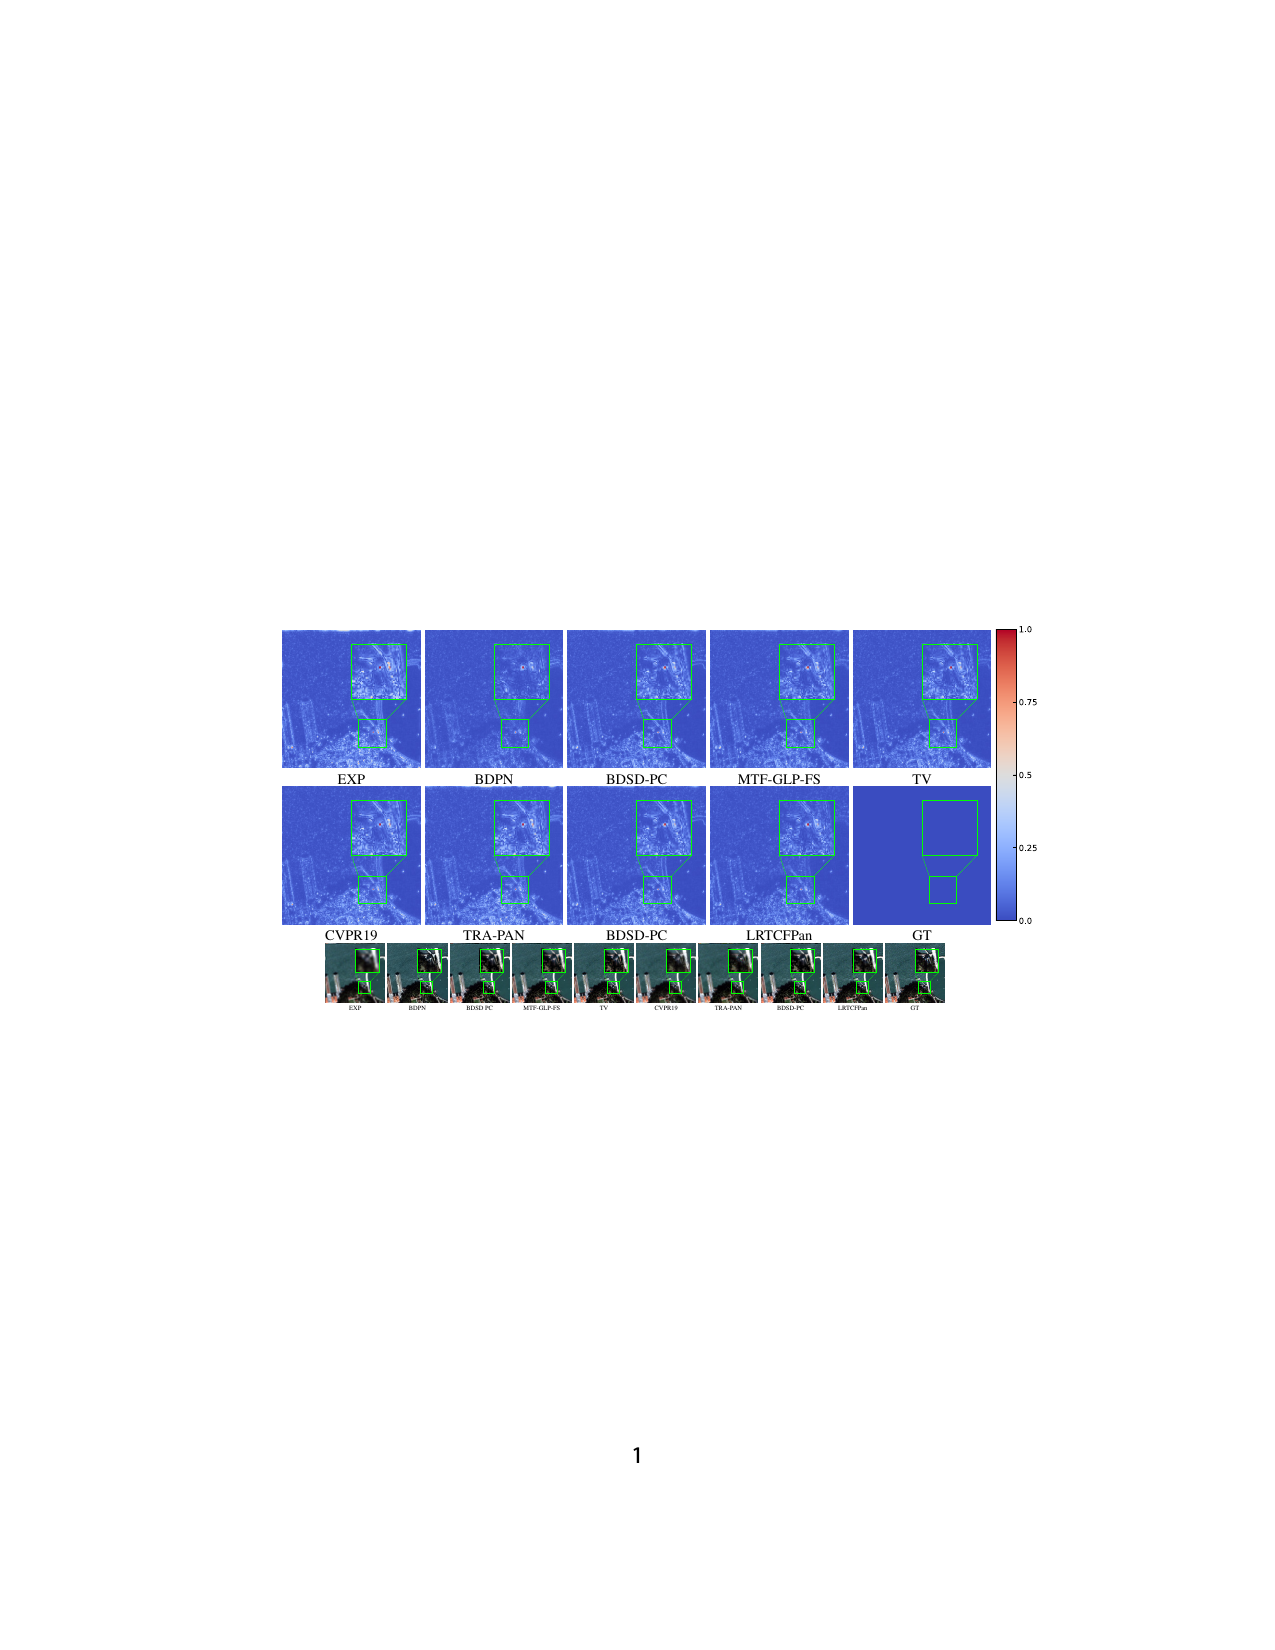}
   \vspace{-20pt}
   \caption{
  Qualitative result comparison between benchmarked methods on the sample image from QB reduced-resolution dataset. The
 first row presents the residual compared to the ground truth, while the second row shows  RGB outputs.
   }
   \vspace{-18pt}
\end{figure*}
