# Supplementary material for: Two-Stage Random Alternation Framework for One-Shot Pansharpening
Source: arXiv:2505.06576 source file (2025-05-16)
Supplement: Supplementary file 2 [file suppl_method.tex]

\begin{table*}[t]
\centering
\vspace{-0.3cm}
\caption{Introduction for pansharpening methods involved in the benchmark.}
\label{tab:methods}
\vspace{-0.1cm}
\begin{tabular}{@{\hskip 3pt}l@{\hskip 3pt}c@{\hskip 3pt}c@{\hskip 3pt}l@{\hskip 3pt}}
\hline
\multirow{2}{*}{\textbf{Method}} & \multirow{2}{*}{\textbf{Category}} & \multirow{2}{*}{\textbf{Year}} & \multirow{2}{*}{\textbf{Introduction}} \\
\hline
EXP~\cite{EXP} & & 2002 & Simply upsamples the MS image. \\
MTF-GLP-FS~\cite{vivoneFullScaleRegressionBased2018} & MRA & 2018 & Estimates the injection coefficients at full resolution rather than reduced resolution. \\
TV~\cite{palssonNewPansharpeningAlgorithm2014} & VO & 2013 & Employs total variation as a regularization technique for addressing an ill-posed problem defined by a commonly utilized explicit model for image formation. \\
BDSD-PC~\cite{vivoneRobustBandDependentSpatialDetail2019} & CS & 2018 & Addresses the limitations of the band-dependent spatial-detail (BDSD) method in images with more than four spectral bands. \\
CVPR2019~\cite{fuVariationalPanSharpeningLocal2019} & VO & 2019 & Integrates a more precise spatial preservation strategy by considering local gradient constraints within distinct local patches and bands. \\
LRTCFPan~\cite{LRTCFPan} & VO & 2023 & Utilizes low-rank tensor completion (LRTC) as the foundation and incorporating various regularizers for enhanced performance. \\
PNN~\cite{masiPansharpeningConvolutionalNeural2016a} & ML & 2016 & The first convolutional neural network (CNN) for pansharpening with three convolutional layers. \\
PanNet~\cite{yangPanNetDeepNetwork2017} & ML & 2017 & Deeper CNN for pansharpening. \\
DiCNN~\cite{hePansharpeningDetailInjection2019} & ML & 2019 & Introduces the detail injection procedure into pansharpening CNNs. \\
FusionNet~\cite{dengDetailInjectionBasedDeep2021} & ML & 2021 & Combines ML techniques with traditional fusion schemes like CS and MRA. \\
DCFNet~\cite{wuDynamicCrossFeature2021} & ML & 2021 & Considers the connections of information between high-level semantics and low-level features through the incorporation of multiple parallel branches. \\
MMNet~\cite{mmnet} & ML & 2022 & A model-driven deep unfolding network with memory-augmentation. \\
LAGConv~\cite{jinLAGConvLocalContextAdaptive2022} & ML & 2022 & Adaptive convolution with enhanced ability to leverage local information and preserve global harmony. \\
HMPNet~\cite{hmpnet} & ML & 2023 & An interpretable model-driven deep network tailored for the fusion of hyperspectral (HS), multispectral (MS), and panchromatic (PAN) images. \\
\hline
\end{tabular}
\vspace{-0.3cm}
\end{table*}
